# Supplementary material for: Fast and Simple Spectral Clustering in Theory and Practice
Source: arXiv:2310.10939 source file (2023-10-17)
Supplement: Supplementary file 1 [file neurips_supplementary.tex]

\documentclass{article}

% if you need to pass options to natbib, use, e.g.:
%     \PassOptionsToPackage{numbers, compress}{natbib}
% before loading neurips_2023

% ready for submission
\usepackage{neurips_2023}

% to compile a preprint version, e.g., for submission to arXiv, add add the
% [preprint] option:
    % \usepackage[preprint]{neurips_2023}

% to compile a camera-ready version, add the [final] option, e.g.:
    % \usepackage[final]{neurips_2023}

% to avoid loading the natbib package, add option nonatbib:
%    \usepackage[nonatbib]{neurips_2023}

\usepackage[utf8]{inputenc} % allow utf-8 input
\usepackage[T1]{fontenc}    % use 8-bit T1 fonts
\usepackage{hyperref}       % hyperlinks
\usepackage{url}            % simple URL typesetting
\usepackage{booktabs}       % professional-quality tables
\usepackage{amsfonts}       % blackboard math symbols
\usepackage{nicefrac}       % compact symbols for 1/2, etc.
\usepackage{microtype}      % microtypography
\usepackage{xcolor}         % colors

% Add custom packages and notation
\usepackage{multirow}
\usepackage{amsmath, amsthm, amssymb}
\usepackage{bm}
\usepackage{subfigure}
\usepackage{wrapfig}
\usepackage[ruled,vlined,linesnumbered]{algorithm2e}
\usepackage{algorithmic}

\usepackage{tikzit}
\usepackage{xr}
\input{basic.tikzstyles}

% Add my commands
\input{notation}

% add cross-reference document
\externaldocument{main}

\title{Fast and Simple Spectral Clustering \\ in Theory and Practice \\ Appendix}

% The \author macro works with any number of authors. There are two commands
% used to separate the names and addresses of multiple authors: \And and \AND.
%
% Using \And between authors leaves it to LaTeX to determine where to break the
% lines. Using \AND forces a line break at that point. So, if LaTeX puts 3 of 4
% authors names on the first line, and the last on the second line, try using
% \AND instead of \And before the third author name.

\begin{document}

\maketitle

\input{sections/appendix}

% \bibliography{references.bib}
\bibliographystyle{plain}

\end{document}
